# Supplementary material for: Guided Flows for Generative Modeling and Decision Making
Source: arXiv:2311.13443 source file (2023-12-07)
Supplement: Supplementary file 1 [file goal_conditioned_appendix.tex]

% \section{Details of the Goal Conditioned Algorithm for Offline RL}
% \label{app:goal_conditioned_algo}
% \begin{figure}[h]
%     \centering
%     \includegraphics[width=0.48\columnwidth]{goal_conditioned_seq_model}
%     \hskip0.1\columnwidth
%     \includegraphics[width=0.4\columnwidth]{idm}\\
%     \caption{Caption}
%     \label{fig:goal_conditioned_seq_model_train}
% \end{figure}
% 
% \begin{figure}[h]
%     \centering
%     \includegraphics[width=0.35\columnwidth]{goal_conditioned_eval}
%     \caption{Caption}
%     \label{fig:goal_conditioned_seq_model_eval}
% \end{figure}
% 
% \begin{algorithm}[h]
% \DontPrintSemicolon
% \small
% \caption{Goal Conditioned Generative Planning}
% \label{algo:planning_goal}
% \textbf{Input:} conditioned sequence model $p_{\theta}(s_t, s_{t+1}, \ldots, s_{t+H-2}, g | s_t, g)$,
% \qq{discuss if we should omit $s_t$ and $g$}
% IDM $f_\rho(s, s')$, 
% initial state $s_0$,
% goal location $g$,
% minimum and maximum number of goal conditioning tokens $n_{\min}$, $n_{\max}$\;
% $t \leftarrow 0$\;
% \While{not done}{
%    \tcp{Progressive Conditioning}
%    $K \leftarrow H - \min(t+n_{\min}, n_{\max})$ \;
%    Sample a sequence $(s_t, \shat_{t+1}, \ldots, \shat_{t+K}=g, \ldots, \shat_{t+H-1} = g) \sim p_\theta(\cdot | s_t, g)$\; % with guidance parameter $\oemga$\;
%    Predict action $\ahat_t = f_\rho(s_t, \shat_{t+1})$\;
%    Execute $\ahat_t$ and observe $s_{t+1}$ and $r_t$\;
%    $t \leftarrow t+1$\;
% }
% \end{algorithm}
% \qq{discuss progressive conditioning}
% 
% \qq{mention hinsight replay, progressive conditioning}
% 
% \qq{multi-goal setup}
% \begin{table}[th]
%     \centering
%     \small 
% \begin{tabular}{c|c|c|c|c}
%     \toprule \hline 
%          & \multicolumn{3}{c|}{\maze} & \multirow{2}{*}{Average}\\ 
%          & \texttt{umaze} & \med & \texttt{large}  & \\ \midrule
%    Flow      & 1.14 &	0.86 & 0.85 & 0.95 \\
%    Diffusion & \highlight{1.27} &	\highlight{1.17} &  \highlight{1.09} & \highlight{1.18}\\
%    \hline \bottomrule 
%     \end{tabular}
%     \caption{Caption}
%     \label{tab:my_label}
% \end{table}
